# Supplementary material for: First constraints on light sterile neutrino oscillations from combined appearance and disappearance searches with the MicroBooNE detector
Source: arXiv:2210.10216 ancillary file (2022-12-06)
Supplement: Supplementary file 1 [file Supplemental_uB_sterileNu.pdf]

# Supplemental Materials for: “First constraints on light sterile neutrino oscillations from combined appearance and disappearance searches with the MicroBooNE detector”

MicroBooNE Collaboration

Figure 1 shows BNB and NuMI neutrino fluxes at MicroBooNE for  $\nu_\mu + \bar{\nu}_\mu$  and  $\nu_e + \bar{\nu}_e$ . The ratios of  $(\nu_\mu + \bar{\nu}_\mu)$  to  $(\nu_e + \bar{\nu}_e)$  are also shown in the bottom panels. The event-weighted average values of this ratio are 185.4 and 25.0 for BNB and NuMI, respectively.

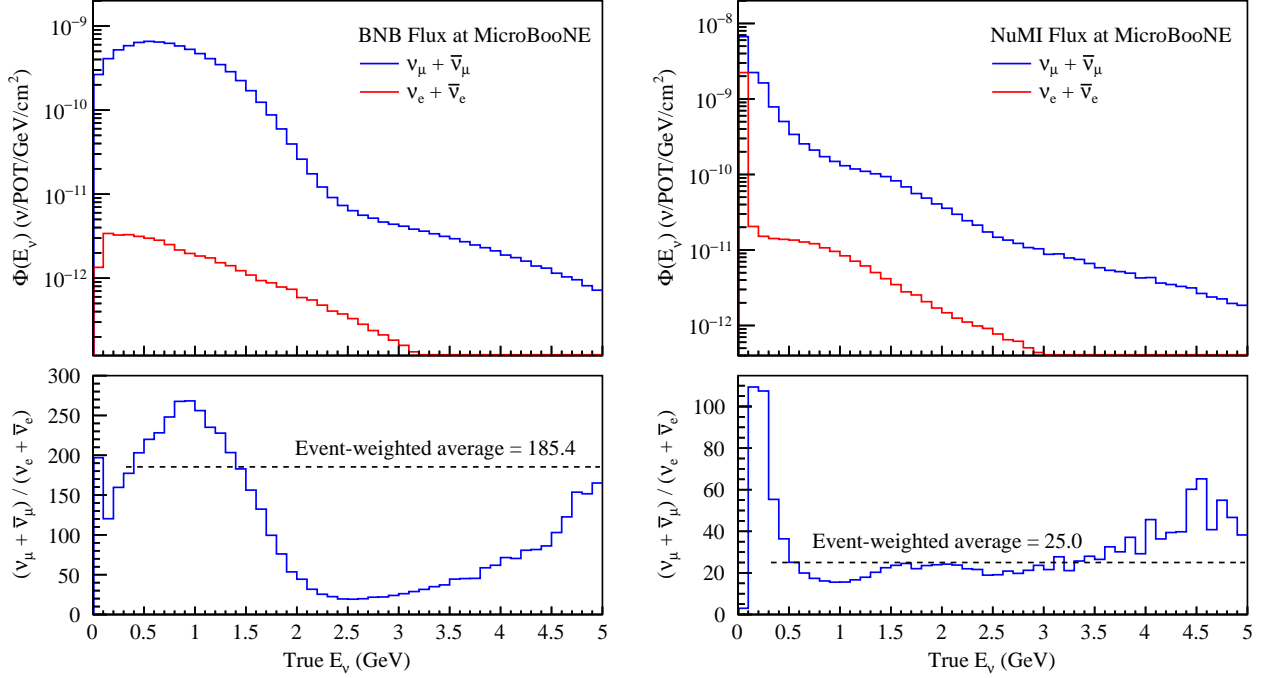

FIG. 1. Intrinsic  $\nu_\mu + \bar{\nu}_\mu$  and  $\nu_e + \bar{\nu}_e$  fluxes as a function of true neutrino energy for BNB (left) and NuMI (right) beams at MicroBooNE in the neutrino mode. The bottom panels show the ratios of  $(\nu_\mu + \bar{\nu}_\mu)$  to  $(\nu_e + \bar{\nu}_e)$ . The event-weighted average of the ratio is calculated by using the events with neutrino energy greater than 300 MeV.

Figure 2 shows the energy spectra of the selected BNB events in the fully contained  $\nu_e$  CC channel for different sets of oscillation parameters. The yellow and blue curves correspond to large oscillation effects, while the red curves show small oscillation effects due to the cancellation between  $\nu_e$  disappearance and appearance when  $\sin^2\theta_{24}$  approaches 0.005.

Figure 3 shows MicroBooNE sensitivity and data exclusion contours at the 95% CL<sub>s</sub> in the planes of  $(\Delta m_{41}^2, \sin^2 2\theta_{\mu e})$  and  $(\Delta m_{41}^2, \sin^2 2\theta_{ee})$  for  $\nu_e$  appearance-only and  $\nu_e$  disappearance-only scenarios. The data and sensitivity differences in both scenarios originate from the overall deficit observed in the  $\nu_e$  CC channels [1].

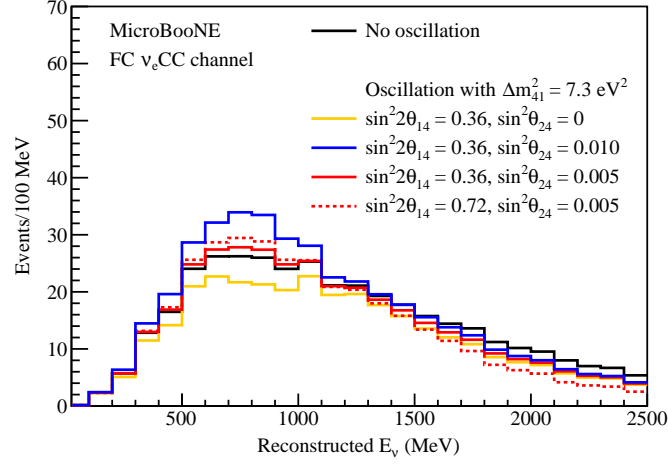

FIG. 2. Energy spectra of the selected events from BNB in the fully contained (FC)  $\nu_e$  CC channel for different sets of oscillation parameters.

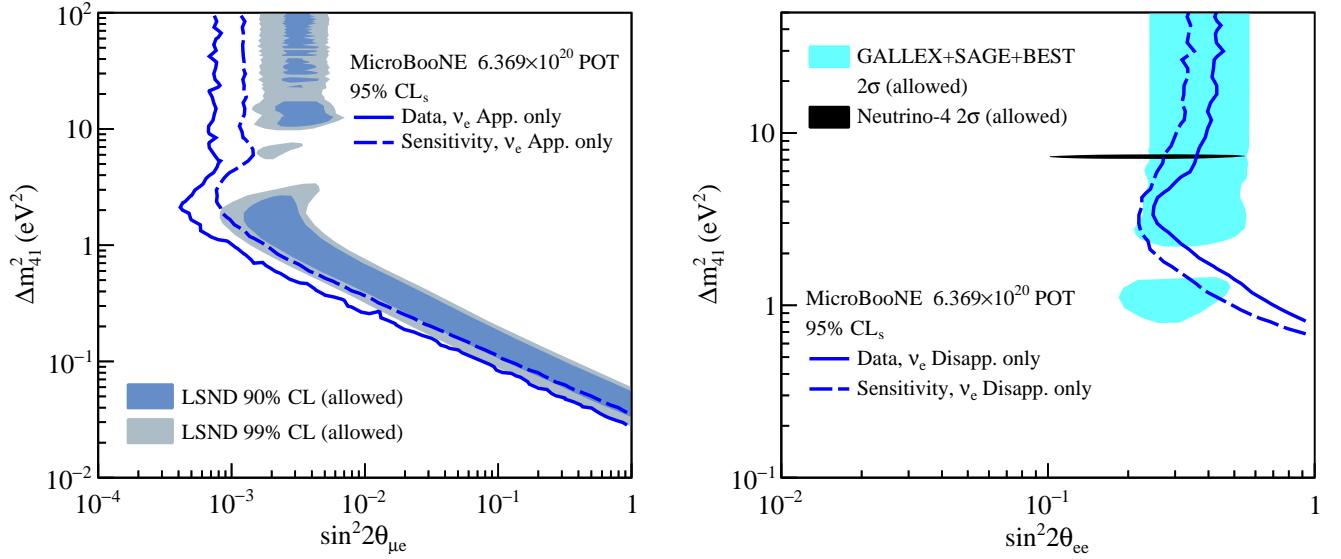

FIG. 3. MicroBooNE  $CL_s$  sensitivity and data exclusion contours at the 95% CL in the plane of  $\Delta m_{41}^2$  and  $\sin^2 2\theta_{\mu e}$  (left) or  $\sin^2 2\theta_{ee}$  (right). The blue solid (dashed) curve represents the MicroBooNE 95%  $CL_s$  data exclusion (Asimov sensitivity) limits in the scenario of  $\nu_e$  appearance-only (left) or  $\nu_e$  disappearance-only (right). In the left figure, the LSND 90% and 99% CL allowed regions [2] using the appearance-only approximation are shown as the light blue and gray shaded areas, respectively. In the right figure, the cyan shaded area represents the  $2\sigma$  allowed region of the gallium anomaly from the experimental results of GALLEX, SAGE, and BEST [3]. The  $2\sigma$  allowed region of the Neutrino-4 experiment [4] is also shown.

- 
- [1] P. Abratenko *et al.* (MicroBooNE Collaboration), Search for an anomalous excess of inclusive charged-current  $\nu_e$  interactions in the MicroBooNE experiment using Wire-Cell reconstruction, Phys. Rev. D **105**, 112005 (2022), arXiv:2110.13978 [hep-ex].
  - [2] A. Aguilar-Arevalo *et al.* (LSND Collaboration), Evidence for neutrino oscillations from the observation of  $\bar{\nu}_e$  appearance in a  $\bar{\nu}_\mu$  beam, Phys. Rev. D **64**, 112007 (2001), arXiv:hep-ex/0104049.
  - [3] V. V. Barinov *et al.*, Results from the Baksan Experiment on Sterile Transitions (BEST), Phys. Rev. Lett. **128**, 232501 (2022), arXiv:2109.11482 [nucl-ex].
  - [4] A. P. Serebrov *et al.*, Search for sterile neutrinos with the Neutrino-4 experiment and measurement results, Phys. Rev. D **104**, 032003 (2021), arXiv:2005.05301 [hep-ex].
